# Supplementary material for: Safe Collective Expression with Social Assurance Contracts
Source: arXiv:2607.05802 source file (2026-09-08)
Supplement: Supplementary file 1 [file safe_coalitions_online_appendix.tex]

\documentclass[safe_coalitions.tex]{subfiles}

\begin{document}

\ifSubfilesClassLoaded{%
  \title{Supplemental Appendix to ``Failure Privacy and Safe Collective Expression''}
  \shortTitle{Supplemental Appendix}
  \issueName{}
  \JEL{}
  \Keywords{}
  \ifanonymizeforpeerreview
    \author{Anonymous}
  \else
    \author{Matthew Cashman\thanks{MIT Sloan, 100 Main Street, Cambridge, MA, USA. Email: \href{mailto:cashman@mit.edu}{cashman@mit.edu}.}}
  \fi
  \date{\today}
  \begin{abstract}
  This Supplemental Appendix contains supporting results, proofs, and extensions for the article.
  \end{abstract}
  \maketitle
}{ }

\startsupplement

\ifSubfilesClassLoaded{ }{%
  \appendixparttitle{Supplemental Appendix}
}

Except in the count-release variant below, the article's terminology applies: to ``name'' an agent is to publish her fixed, identity-bound statement, report, or other expression. A public roster records whose expressions have been published; it is not an announcement followed by a later choice to act.

\section{Count Release: Supporting Result}\label{sec:count_release}

This section records the count-release variant of the tunnel used in the applications. The practical trigger is an authenticated total count or a small vector of preannounced class-count quotas. The general protection-family rule identifies the greatest safe roster conditional on the supplied requirements. It does not claim that a platform can elicit or evaluate arbitrary requirements that depend on roster composition.

\paragraph{Count release.} Some deployed mechanisms release a \emph{number} rather than jointly publishing statements under their authors' identities. The protective audience receives an authenticated count of sealed authorizations, while the retaliating audience sees no name even on success. Call a mechanism \emph{count-release} if it holds completed authorizations as before but publishes only the certified mass of the released coalition. The roster goes only to the certifier, who is bound to keep it confidential. In the scalar benchmark, protection depends on mass: the threshold families $\Pfam_i=\{C\ni i: b+m(C)\ge\rho_i\}$ are upper sets in mass and do not depend on identities. The certified count is therefore the statistic on which the rule conditions. Whether that certificate protects a later individual act lies outside the proposition.

\begin{proposition}[Count release]\label{prop:count}
In the nonatomic scalar benchmark with the threshold families above:
\begin{enumerate}
\item[(i)] The threshold families are upper sets in mass, so Assumption~\ref{ass:M} holds and Theorems~\ref{thm:largest} and~\ref{thm:cascade} apply. Their least and greatest fixed points take the scalar form in equation~\eqref{eq:granovetter}: $\Cs$ and $\Cp$ collect the consenters with requirements at or below $y^-$ and $y^+$.
\item[(ii)] Conditional on $V=S$, the tunnel rule with count-only publication assembles and certifies the same mass $y^+$. Because count release never names an agent, the paper's naming-based safety requirement is vacuously satisfied. The rule certifies only masses for which $b+m\ge\rho_i$ for every member of $D(V)$. This self-protecting-roster calculation determines the mass certified but does not establish that the certificate protects a later self-identifying act, which lies outside the mechanism. The proposition assumes private accumulation and therefore does not cover observable signing. The companion paper discusses related exposure and observability risks, but neither paper solves a general observable-signing equilibrium \citep{cashmanConditionalDisclosureCoordination}. Mere certifier knowledge is not a harmful leak. A breach that transmits an under-protective roster to the retaliating audience instead enters the harmful-breach term $\delta_i^{\mathrm h}$ in Proposition~\ref{prop:robust_frontier}.
\item[(iii)] Theorem~\ref{thm:necessity} concerns histories that enlarge the public named coalition, which count release never does. Count release still uses completed private authorizations; it changes the released object from names to certified mass. It is therefore not a public-only route past $\Cs$. Publishing only a count withholds the roster mechanically but does not guarantee anonymity. A small candidate set can concentrate the audience's posterior, an exact certified mass can identify a unique roster when masses are atomic, and a count equal to the whole candidate population identifies everyone. Inference depends on candidate sets, side information, and priors that the model does not track.
\end{enumerate}
\end{proposition}

\begin{proof}[Proof of Proposition~\ref{prop:count}]
(i) Inclusion weakly increases mass. Thus $C\in\Pfam_i$ and $C\subseteq C'\ni i$ imply $C'\in\Pfam_i$, so Assumption~\ref{ass:M} holds. Equation~\eqref{eq:granovetter} gives the fixed-point specialization; finite-step attainment becomes monotone convergence in the nonatomic benchmark.

(ii) Run $D(V)=\Cp(V)$ with the publication map replaced by the certified mass $b+m(D(V))$. No history names anyone to the retaliating audience, so Assumption~\ref{ass:RES} imposes no naming restriction. Conditional on $V=S$, the certified mass is $b+m(\Cp(S))=y^+$, with $\Cp(S)$ self-protecting by Theorem~\ref{thm:largest}. The rule certifies only self-protecting masses, so $b+m(D(V))\ge\rho_i$ for every $i\in D(V)$. Whether that certificate protects an agent who later identifies herself, and the later act itself, lie outside the mechanism.

(iii) Both parts of Theorem~\ref{thm:necessity} concern histories at which agents become newly \emph{named}. Part (i) bounds the public named set, while part (ii) derives the private stage from the transition that first names an unsafe agent. Count release has no such history. It uses the same holding stage for a different object, a mass certificate.
\end{proof}

\section{The Fight-or-Fold Opponent: Per-Member Result}\label{app:opponent}

The fight-or-fold model in Section~\ref{sec:target} treats retaliation as all-or-none. This section shows that its reversal survives when the opponent makes the punishment decision member by member. Punishing one member of a released coalition of mass $m$ costs $\kappa_T \psi(m)$, with $\psi$ continuous, strictly increasing, and positive. Punishment prevents the fixed harm $d_i>0$ that member $i$'s participation would impose on the opponent. The opponent therefore punishes $i$ exactly when $d_i\ge\kappa_T \psi(m)$. Its cost type $\kappa_T$ is drawn once from a continuous, strictly increasing cdf $\Lambda$ with full support on $(0,\infty)$. A punished member's expression is suppressed; an unpunished member's expression stands.

\begin{proposition}[Per-member reversal and selective retaliation]\label{prop:permember}
Let $p_i(m)=\Lambda\!\big(d_i/\psi(m)\big)$ be the probability that member $i$ of a released mass-$m$ coalition is punished, let $h_i>0$ and $e_i\ge0$, and let $i$ accept release iff $e_i\ge p_i(m)\,h_i$. Then: (i) acceptance is a mass threshold: $i$ accepts iff $m\ge\mu_i$. When $e_i=0$, $\mu_i=\infty$. When $0<e_i<h_i$, $\mu_i=\psi^{-1}\!\big(d_i/\Lambda^{-1}(e_i/h_i)\big)$. If the argument exceeds $\psi$'s range, set $\mu_i=\infty$, so the agent never accepts; if it falls below the range, set $\mu_i=0$. When $e_i\ge h_i$, $\mu_i=0$. At a common tolerance $e/h$, the cutoff $\mu_i$ is weakly increasing in $d_i$. The induced protection families are upward sets, and $\Cs,\Cp$ exist by Lemma~\ref{lem:interim}; (ii) for every hidden supporter $i\in\Cp\setminus\Cs$, replacing open organizing with release of $\Cp$ raises observed retaliation on her from $0$ to $p_i(m(\Cp))\in(0,1)$ and lowers suppression of her expression from $1$ to the same interior number: the reversal holds member by member; (iii) every already-visible member $j\in\Cs$ is punished with weakly lower probability after the release, $p_j(m(\Cp))\le p_j(m(\Cs))$; (iv) at any released mass, punishment concentrates on the most damaging members: $p_i(m)$ is increasing in $d_i$.
\end{proposition}

\begin{proof}[Proof of Proposition~\ref{prop:permember}]
(i) $e_i\ge p_i(m)h_i$ iff $\Lambda(d_i/\psi(m))\le e_i/h_i$. If $e_i=0$, the left side is false at every finite mass because $d_i/\psi(m)>0$ and full support makes $\Lambda(d_i/\psi(m))>0$, so $\mu_i=\infty$. If $e_i\ge h_i$ the inequality holds for every $m$ since $\Lambda\le1$. For $0<e_i<h_i$, $\Lambda$ continuous and strictly increasing with full support gives: acceptance iff $d_i/\psi(m)\le\Lambda^{-1}(e_i/h_i)$, i.e., iff $\psi(m)\ge d_i/\Lambda^{-1}(e_i/h_i)$, a mass threshold $\mu_i$ increasing in $d_i$ and decreasing in $e_i/h_i$. Acceptance sets are upward in mass, hence upward in inclusion, and Lemma~\ref{lem:interim} delivers the lattice objects. (ii) Under open organizing a hidden supporter never surfaces: no punishment against her can be recorded, and her expression never stands, so observed retaliation is $0$ and suppression is $1$. Under release of $\Cp$, which is self-protecting under the induced families, she accepts and is punished iff $\kappa_T\le d_i/\psi(m(\Cp))$, an event of probability $p_i(m(\Cp))=\Lambda(d_i/\psi(m(\Cp)))\in(0,1)$ because $d_i>0$ and $\Lambda$ is interior on $(0,\infty)$. Her expression is suppressed exactly when she is punished. Observed retaliation thus rises from $0$ to $p_i(m(\Cp))$ while suppression falls from $1$ to $p_i(m(\Cp))$. (iii) $m(\Cp)\ge m(\Cs)$ and $\psi$ increasing give $d_j/\psi(m(\Cp))\le d_j/\psi(m(\Cs))$; apply $\Lambda$. (iv) Immediate since $\Lambda$ is increasing.
\end{proof}

The coalition-level fight-or-fold choice in eq.~\ref{eq:fold} is the constrained case in which punishment must be all-or-none. The per-member model shows that the reversal does not depend on that constraint, and part (iv) gives the selective-discharge pattern documented in the union evidence. The proposition also shows that the minimum coalition mass at which a member accepts release, $\mu_i$, rises with the harm $d_i$ she imposes on the opponent.

The observable-attempt comparative static below uses one fixed-point lemma.

\begin{lemma}[Shifted crossings]\label{lem:shift}
Let $b\le M$ and let $G,\tilde G:[b,M]\to[b,M]$ be nondecreasing with $\tilde G\le G$ pointwise and $G(b)\ge b$, $\tilde G(b)\ge b$.
\begin{enumerate}
\item[(i)] (\emph{Monotonicity.}) Least fixed points exist (Tarski), and $\mathrm{lfp}(\tilde G)\le\mathrm{lfp}(G)$.
\item[(ii)] (\emph{Continuity.}) Let $\{G_s\}_{s\in[0,\bar s]}$ be pointwise nonincreasing in $s$, with each $G_s$ continuous on $[b,M]$ and $(y,s)\mapsto G_s(y)$ jointly continuous. Then $s\mapsto\mathrm{lfp}(G_s)$ is nonincreasing and right-continuous, and it is continuous at any $s_0$ at which the least fixed point is a \emph{transversal} crossing---$G_{s_0}<\mathrm{id}$ on an interval immediately above $\mathrm{lfp}(G_{s_0})$. Without transversality, a new fixed point can appear by tangency below the previous least fixed point, causing a downward discontinuity from the left.
\end{enumerate}
\end{lemma}

\begin{proof}[Proof of Lemma~\ref{lem:shift}]
(i) For nondecreasing $G$ on the complete lattice $[b,M]$, Tarski gives $\mathrm{lfp}(G)=\inf\{y:G(y)\le y\}$; the set is nonempty because $G(M)\le M$. Since $\tilde G\le G$, every pre-fixed point of $G$ is a pre-fixed point of $\tilde G$, ordering the infima. (ii) Monotonicity is (i). Write $\ell(s)=\mathrm{lfp}(G_s)$, which is nonincreasing. Fix $s_0$ and $\eta>0$. For $y<\ell(s_0)$, $G_{s_0}(y)>y$, so $G_{s_0}-\mathrm{id}$ has a positive minimum on the compact $[b,\ell(s_0)-\eta]$ when it is nonempty. Joint continuity keeps $G_s>\mathrm{id}$ there for $s$ near $s_0$, whence $\ell(s)>\ell(s_0)-\eta$; with monotonicity this gives right-continuity. Under transversality, choose $y^*\in(\ell(s_0),\ell(s_0)+\eta)$ with $G_{s_0}(y^*)<y^*$. Joint continuity keeps $G_s(y^*)<y^*$ nearby, so $\ell(s)\le y^*<\ell(s_0)+\eta$. The bounds give continuity. A tangency below the running least fixed point shows why transversality cannot be dropped.
\end{proof}

\section{Frontier Supporting Results}\label{sec:frontier_supp}

This section states and proves the interim bounds and the observable-attempt comparative static summarized in the article.

\begin{proposition}[Necessity at positive tolerance]\label{prop:interim_necessity}
(i) If $\Cs(S)\subsetneq\Cp(S)$ and $r_i\ge 1-(1-\varepsilon)^{|B|}$ for every agent $i$ of the nonempty batch $B=\Cp(S)\setminus\Cs(S)$, a single unverified synchronized public batch is acceptable to every member and realizes $\Cp(S)$ with probability $(1-\varepsilon)^{|B|}>0$: with tolerant participants, a private stage is not necessary to reach beyond the cascade. (ii) Fix a mechanism and agent $i$. Let $X_i$ be the event that $i$ is exposed. Suppose that at a trigger $h$, reached before the same-date completion draws, $i$ is not safe with the current public set alone and her own exposure attempt rests on an unverified batch $B_h\ne\varnothing$. Let $H_{ih}$ be the event that $h$ is reached and $i$'s attempt completes, and write $\alpha_{ih}=\Pr(H_{ih}\mid X_i)$. Then
\[
\Pr(i\text{ is exposed unprotected}\mid X_i)\ \ge\ \alpha_{ih}\varepsilon^{|B_h|}.
\]
Consequently acceptability requires $\alpha_{ih}\varepsilon^{|B_h|}\le r_i$. For pairwise disjoint trigger events, the corresponding lower bounds add. Safe exposure on other branches can make $\alpha_{ih}<1$, so $r_i<\varepsilon^{|B_h|}$ alone does not rule out the trigger. (iii) At the exact endpoint $r=0$, every positive-mass not-yet-safe unverified trigger is excluded; interim acceptability is regret-freeness and Theorem~\ref{thm:necessity} applies. Along any sequence of acceptable mechanisms with $r^n\to0$, each agent's mechanism-wide unprotected-exposure risk converges to zero, although it may remain positive at every $n$.
\end{proposition}

\begin{proof}[Proof of Proposition~\ref{prop:interim_necessity}]
(i) Let $B=\Cp(S)\setminus\Cs(S)$ be announced and attempted at once from the public state $\Cs(S)$. For $i\in B$, conditional on her own completion, the realizations leaving her unprotected are contained in the event that not all of $B\setminus\{i\}$ complete, of probability $1-(1-\varepsilon)^{|B|-1}\le1-(1-\varepsilon)^{|B|}\le r_i$, so she accepts; if all complete, the realized public set is $\Cp(S)\in\Pfam_i$ for every member, an event of probability $(1-\varepsilon)^{|B|}$.

(ii) Condition on $X_i$. On $H_{ih}$, completion independence gives probability $\varepsilon^{|B_h|}$ that every member of $B_h$ fails. In that realization $i$ is named in the current public set plus herself, which is outside $\Pfam_i$ by hypothesis. Hence the harmful event has conditional probability at least $\Pr(H_{ih}\mid X_i)\varepsilon^{|B_h|}=\alpha_{ih}\varepsilon^{|B_h|}$. Acceptability yields the inequality, and disjoint trigger events can be summed. Safe exposure on other branches lowers this trigger's share of agent $i$'s total exposure, making $\alpha_{ih}<1$, but does not change the probability that every member of $B_h$ fails at the trigger.

(iii) At $r=0$, part (ii) rules out every unverified not-yet-safe trigger with $\alpha_{ih}>0$. Every completion pattern has positive probability, so zero mechanism-wide risk is regret-freeness on almost every branch of the mechanism's randomization; Theorem~\ref{thm:necessity} then applies. Along $r^n\to0$, acceptability directly bounds each mechanism-wide conditional risk by $r_i^n$, proving convergence without exact zero at any positive tolerance.
\end{proof}

Now suppose failed attempts may be observed. Each \emph{failed} attempt is observed by the retaliating audience with probability $\omega\in[0,1]$, independently across attempts. Observing one unit of failed-attempt mass raises each still-private consenter's future requirement by $\xi\ge0$, but it does not change the protection of agents already named. The process follows the greedy path in Theorem~\ref{thm:selection} with the completion model of Proposition~\ref{prop:interim_necessity}. Each attempt completes independently with probability $1-\varepsilon$ and is retried until it completes, so each unit of completed mass generates $\varepsilon/(1-\varepsilon)$ units of failed attempts in expectation. The fluid benchmark evaluates accumulated failures at this expectation. Building public mass $y$ from the seed then raises future requirements by $\lambda(\omega)\,(y-b)$, where $\lambda(\omega)=\omega\xi\varepsilon/(1-\varepsilon)$. A consenter with requirement $\rho_i$ is safe to join at mass $y$ iff $y\ge\rho_i+\lambda(\omega)(y-b)$. The curve in equation~\eqref{eq:granovetter} becomes
\[
G^{\omega}_S(y)\;=\;b+H_S\bigl((1-\lambda(\omega))\,y+\lambda(\omega)\,b\bigr),
\qquad \lambda(\omega)<1,
\]
still nondecreasing in $y$, and pointwise weakly falling in $\omega$.

\begin{proposition}[Observability and the stall]\label{prop:observability}
Consider the scalar nonatomic benchmark, in which $H_S$ is continuous, and use the fluid interpretation above. Maintain the baseline crossing configuration used for the targeted pact: $y^-<y^u<y^+$ and $G_S<\mathrm{id}$ on $(y^-,y^u)$. Let $\lambda(\omega)=\omega\xi\varepsilon/(1-\varepsilon)<1$, with observed failures affecting only future requirements:
\begin{enumerate}
\item[(i)] (\emph{The stall moves down; no jump at the onset.}) The open greedy path stalls at $y^-(\omega)$, the least fixed point of $G^{\omega}_S$ above the seed. On the range of $\omega$ with $\lambda(\omega)<1$, $y^-(\omega)$ is nonincreasing in $\omega$ (and in $\xi$, and in $\varepsilon$ through $\lambda$), right-continuous, and continuous at every $\omega$ whose stall is a transversal crossing---$G^{\omega}_S<\mathrm{id}$ immediately above $y^-(\omega)$---as at $\omega=0$, where the standing configuration puts $G_S<\mathrm{id}$ on $(y^-,y^u)$; at an interior $\omega$ where the rescaled curve instead touches the diagonal below the running stall, $y^-(\omega)$ can step down discretely (Lemma~\ref{lem:shift}(ii)). $y^-(0)=y^-$ recovers Theorem~\ref{thm:selection}'s stall exactly, as does $\xi=0$ (observed failures do not raise future requirements) or $\varepsilon=0$ (nothing fails, so nothing is seen).
\item[(ii)] (\emph{Marginal erosion.}) If $H_S$ is continuously differentiable near $y^-$ with $H_S'(y^-)<1$, then
\[
\frac{dy^-}{d\omega}\Big|_{\omega=0}
=\;-\,\frac{\xi\varepsilon}{1-\varepsilon}\cdot
\frac{H_S'(y^-)\,\bigl(y^--b\bigr)}{1-H_S'(y^-)}\;\le\;0,
\]
strict whenever $\xi\varepsilon>0$, $H_S'(y^-)>0$, and $y^->b$: the stall prediction degrades smoothly in the observability of failure, not discretely.
\end{enumerate}
\end{proposition}

When $\omega>0$, a failed attempt raises the future requirements faced by the attempter and everyone else. The costless-failure condition in Theorem~\ref{thm:selection} therefore fails. The proposition characterizes the fluid greedy path, not equilibrium selection for $\omega>0$. Equilibrium analysis and the finite-population stochastic path remain open.

\begin{proof}[Proof of Proposition~\ref{prop:observability}]
(i) For $\lambda<1$, the map $y\mapsto(1-\lambda)y+\lambda b$ is increasing. Hence $G^\omega_S$ is nondecreasing and maps $[b,\,b+m(S)]$ into itself, with $G^\omega_S(b)=b+H_S(b)\ge b$. For $y\ge b$, its argument $(1-\lambda)y+\lambda b=y-\lambda(y-b)$ is nonincreasing in $\lambda$. The parameter $\lambda$ is increasing in $\omega$, $\xi$, and $\varepsilon$ on $[0,1)$, so $G^{\omega}_S$ is pointwise nonincreasing in each of them because $H_S$ is nondecreasing.

The condition $y\ge\rho_i+\lambda(y-b)$ is equivalent to $\rho_i\le(1-\lambda)y+\lambda b$. Because $\lambda<1$, the right-hand threshold rises along the path. The mass joined by $y$ is therefore $H_S((1-\lambda)y+\lambda b)$, and the fluid open path iterates $G^\omega_S$ from the seed. Continuity of $H_S$ implies convergence to $y^-(\omega)=\mathrm{lfp}(G^\omega_S)$. In the nonatomic round-by-round process, a joiner's own failed attempts have zero mass, and expected cumulative requirement increases after each round equal $\lambda$ times completed mass. Thus iteration of $G^\omega_S$ is exact for this fluid recursion.

Lemma~\ref{lem:shift}(i)--(ii) now gives monotonicity and continuity; joint continuity in $(y,\omega)$ follows by composition. At $\omega=0$, the stall is transversal because $G_S<\mathrm{id}$ on $(y^-,y^u)$. At an interior $\omega$, transversality must be checked for $G^{\omega}_S$ at its new stall. It does not follow from the benchmark because $y^-(\omega)$ may move into the region where $G_S>\mathrm{id}$. If the graph of $H_S$ is tangent below the stall to the ray with slope $1/(1-\lambda)$, the least fixed point moves down discretely. The continuity claim therefore applies exactly at transversal values of $\omega$. At $\lambda=0$, the curve is $G_S$ and its least fixed point is $y^-$. (ii) $F(y,\lambda)=y-b-H_S((1-\lambda)y+\lambda b)$ is $C^1$ near $(y^-,0)$ with $F_y=1-H_S'(y^-)>0$ there, so the implicit function theorem gives a $C^1$ branch of solutions through $(y^-,0)$, which coincides with $\lambda\mapsto y^-(\lambda)$ near $0$ by (i)'s continuity and the branch's local uniqueness. Differentiating along it: $\dot y=H_S'(y^-)\bigl[(b-y^-)+\dot y\bigr]$, so $\dot y=-H_S'(y^-)(y^--b)/(1-H_S'(y^-))$, and $d\lambda/d\omega=\xi\varepsilon/(1-\varepsilon)$.
\end{proof}

\section{Act-Space Representation and Risk--Reach Details}\label{sec:representation_details}

This section states the scope conditions used in Section~\ref{sec:necessity}. Attribution is always relative to an audience. An act that reveals an attribute without identifying a participant does not enlarge the public coalition; it instead changes beliefs or future protection requirements, as in Proposition~\ref{prop:observability}. An identity event carried by no completed act is a breach and enters the harmful-leak rate of Proposition~\ref{prop:robust_frontier}. Environment E1 holds the protection families fixed and lets payoffs depend on the public-coalition path, released sets, and an agent's own private act costs. Legal protection, insurance, or belief campaigns that change the families are environment interventions; the results apply at the families they induce.

Lemma~\ref{lem:dichotomy} represents only acts with deterministic attribution. Splitting one stochastically attributed act into simultaneous exposure and commitment acts would conflict with the primitive that every subset of attempted actions may complete. The split would add a both-complete realization absent from the original lottery. Stochastic attribution is therefore a risk extension, not an exact same-act equivalence. At zero tolerance every positive-probability attributing outcome must itself be safe; at positive tolerance its probability enters the participant's unprotected-exposure risk. Neither observation licenses the stronger two-type representation, which the paper does not claim.

Lemma~\ref{lem:holding} allows the device to be a person. A colleague who publishes a co-signed letter is a holding stage if she first receives the others' completed, unattributed authorizations and conditions her release act on them. The reach of that informal tunnel is limited by trust in the delegate rather than by a platform's scale. A merely correlated set of separate attempts is different: unless the institution eliminates every proper-subset realization, unilateral completion remains in the set of admissible outcomes. Correlation can lower expected risk at positive tolerance but cannot create exact joint completion at zero tolerance.

The trigger comparison in Theorem~\ref{thm:dominance}(i) is local. At public state $C$, suppose an acceptable mechanism rests $i$'s unsafe exposure on same-date attempts by $B_i$. Its completed-authorization replacement solicits the same agents until all authorizations are held and then releases $T=C\cup\{i\}\cup B_i$ as one act. The local comparison assumes this full-completion target protects every trigger participant not already safe in $C$; whole-mechanism acceptability does not imply that condition when an agent can be exposed on several branches. The replacement exposes no one before the protecting release, while the original leaves $i$ unprotected when her act completes and every act in $B_i$ fails, an event of probability $(1-\varepsilon)\varepsilon^{|B_i|}$ conditional on reaching the trigger, or $\varepsilon^{|B_i|}$ conditional additionally on $i$'s completion. On shared draws the replacement's released set contains every agent the original trigger exposes. Without retries, however, strict conditionality discards partial batches and the reach comparison fails.

Three limits prevent this local replacement from proving the global result by iteration. First, in a one-shot environment a partially completed unverified batch may protect and expose more agents than a conditional release that fails. Second, at $r_i\ge1$ an agent accepts certain unprotected exposure and acts as an endogenous seed, allowing acceptable reach outside $\Cp(S)$. Third, replacing one trigger can increase entry into downstream states and thereby amplify third-party risk, or remove unsafe exposures that served as stepping stones. Theorem~\ref{thm:dominance}(ii) therefore uses the whole-mechanism confinement bound rather than iterating part (i). Act costs and delay are also outside its two-coordinate comparison and enter through the entry problem.

\section{Relation to Dynamic Coordination}\label{sec:gale}

The cascade shares \citet{galeMonotoneGamesPositive2001}'s primitives: actions are nondecreasing, irreversible, and publicly observed, with positive spillovers. The comparison nevertheless requires a payoff completion. The protection families determine only the sign of payoffs at binary rosters, whereas Gale's characterization is for continuous payoffs on interval action spaces. The next result supplies that bridge rather than treating the binary environment as an automatic specialization.

\begin{proposition}[A Gale completion versus regret-free safety]\label{prop:gale}
Maintain Assumption~\ref{ass:M}, let $P=\Cp(S)$ be nonempty, and set $n=|P|$. There exists an auxiliary continuous positive-spillover game on $[0,1]^P$ such that:
\begin{enumerate}
\item[(i)] at every binary roster $C\subseteq P$, an exposed agent's terminal payoff is positive if $C$ protects her and negative otherwise, while abstention pays zero;
\item[(ii)] full exposure $\mathbf 1_P$, corresponding to $P$, is the unique SPE limit of Gale's monotone game;
\item[(iii)] under Assumption~\ref{ass:U}, the maximal roster reachable by regret-free public exposure remains $\Cs(S)$. Hence, if $\Cs(S)\subsetneq\Cp(S)$, a continuous terminal-payoff equilibrium can reach the tunnel destination, while a public path safe at every exposure cannot.
\end{enumerate}
\end{proposition}

\begin{proof}[Proof of Proposition~\ref{prop:gale}]
Fix $\eta\in(0,1/(n+1))$. For $i\in C\subseteq P$, define the binary terminal payoff
\[
v_i(C)=
\begin{cases}
1+\eta|C|,&C\in\Pfam_i,\\
-1+\eta|C|,&C\notin\Pfam_i.
\end{cases}
\]
For $x\in[0,1]^P$, let $R_{-i}(x)$ include each $j\ne i$ independently with probability $x_j$, and set
\[
u_i(x)=x_i\,\mathbb E\!\left[v_i\bigl(\{i\}\cup R_{-i}(x)\bigr)\right].
\]
This multilinear extension is continuous. At a binary corner $\mathbf 1_C$, it gives zero to $i\notin C$ and $v_i(C)$ to $i\in C$; because $\eta n<1$, the latter is positive exactly when $C\in\Pfam_i$. Adding another agent raises $v_i$ by $\eta$ if protection is unchanged and by $2+\eta$ if protection switches from unsafe to safe. Assumption~\ref{ass:M} rules out the reverse switch, so $u_i$ is nondecreasing in every other player's action: the completion has positive spillovers.

Since $P$ is self-protecting, $u_i(\mathbf 1_P)=1+\eta n$ for every $i$. If $x\ne\mathbf 1_P$, then every player's payoff is strictly below $1+\eta n$: this follows immediately for $x_i<1$; when $x_i=1$, some $j\ne i$ has $x_j<1$, and the strictly positive $\eta$ increment from $j$ makes the expectation strictly smaller. Thus $\mathbf 1_P$ strictly Pareto-dominates every other action profile, and in particular every other \emph{satiation point}, a profile from which no player can gain by increasing her own action. \citet[Theorem~3]{galeMonotoneGamesPositive2001} therefore makes $\mathbf 1_P$ the unique SPE limit on these bounded interval action spaces. For part (iii), every safe-expansion iterate is self-protecting and hence is contained in $P$ by Theorem~\ref{thm:largest}; restricting the comparator's player set to $P$ therefore preserves the original cascade endpoint. Theorem~\ref{thm:cascade}(i)--(ii) gives the claim.
\end{proof}

The completion is an existence benchmark, not a behavioral identification claim. A fractional $x_i$ is an irreversible participation-probability or intensity commitment, and the small $\eta|C|$ term deliberately creates strict Pareto dominance. Selection of $\Cp$ therefore does not follow from the paper's ordinal protection primitives alone. The construction shows the narrower point the comparison needs: when only the terminal roster enters payoffs, equilibrium continuation can support the greatest safe destination even though some intermediate rosters are unsafe. The paper's regret-free requirement requires protection at every exposure and therefore stops the public path at $\Cs$. Conditional release restores the terminal destination without asking agents to trust future action by others: it substitutes completed private authorization and joint release for equilibrium continuation (Theorem~\ref{thm:necessity}).

\section{Heterogeneity and the Difference in Reach}\label{sec:gap}

Outside the homogeneous case, the protection-requirement distribution determines the difference between the cascade and tunnel. The results below give the heterogeneous fixed-point geometry and comparative statics used in the article. Let $H_S(y)=m\{i\in S:\rho_i\le y\}$ and $G_S(y)=b+H_S(y)$. Let $y^-\le y^+$ be the least and greatest fixed points of $G_S$, the public masses of $\Cs$ and $\Cp$ in the scalar specialization of Theorems~\ref{thm:largest} and~\ref{thm:cascade}. The companion paper separately studies how signing frictions affect entry in a homogeneous population \citep{cashmanConditionalDisclosureCoordination}.

\begin{proposition}[Exposure barriers and the difference in reach]\label{prop:gap}
In the scalar nonatomic benchmark, with continuous $H_S$:
\begin{enumerate}
\item[(i)] the contribution is the fixed-point distance, $m(\Cp)-m(\Cs)=y^+-y^-$;
\item[(ii)] (\emph{Exposure barriers.}) The inequality $y^-<y^+$ is equivalent to $G_S$ having multiple fixed points. An \emph{exposure barrier}---a level $y>y^-$ at which the protected mass falls short of the mass needed to sustain it, $G_S(y)<y$, with a recrossing above it ($G_S(y')\ge y'$ for some $y'>y$)---is sufficient for $y^-<y^+$ and is also necessary when the lower endpoint is \emph{locally blocked} ($G_S(y)<y$ for all $y$ in a right-neighbourhood of $y^-$). Without local blockage, multiple fixed points can instead arise through a critical-mass or tangency case, in which the cascade endpoint is not robust to an upward perturbation but no exposure barrier separates it from $y^+$;
\item[(iii)] raising $H_S$ only on $(y^-,\infty)$ leaves $y^-$ (hence $\Cs$) unchanged and weakly raises $y^+$ (hence $\Cp$); raising $H_S$ on $[b,y^-]$, or raising the seed $b$, weakly raises $y^-$.
\end{enumerate}
\end{proposition}

\begin{proof}[Proof of Proposition~\ref{prop:gap}]
(i) $\Cp=\{i:\rho_i\le y^+\}$ and $\Cs=\{i:\rho_i\le y^-\}$, so $m(\Cp)=H_S(y^+)=y^+-b$ and $m(\Cs)=H_S(y^-)=y^--b$ at the fixed points; subtract. (ii) The condition $y^-<y^+$ means that $G_S$ has two distinct fixed points, directly from the definitions of $y^-\le y^+$. \emph{Sufficiency}: let $y_0>y^-$ satisfy $G_S(y_0)<y_0$ with $G_S(y')\ge y'$ for some $y'>y_0$. Since $G_S$ is continuous in the nonatomic benchmark, the intermediate value theorem gives a fixed point in $(y_0,y']$, so $y^+>y_0>y^-$. \emph{Necessity under local blockage}: if $y^-<y^+$ and $G_S(y)<y$ on $(y^-,y^-+\varepsilon)$, any $y_0\in(y^-,\,y^-+\min\{\varepsilon,\,y^+-y^-\})$ has $G_S(y_0)<y_0$ and recrosses at $y'=y^+$, an exposure barrier. Local blockage cannot be dropped: for $b=1$, $G_S(y)=1+\sqrt{y-1}$ on $[1,2]$, the fixed points are $1$ and $2$, yet $G_S(y)>y$ throughout $(1,2)$. Thus $y^-<y^+$ without an exposure barrier. Here $y^-=b$, the cascade never leaves the seed, and any upward perturbation at the unstable lower fixed point can start it. (iii) The iteration to $y^-$ evaluates $G_S$ only at masses $\le y^-$, so $y^-$ depends only on $H_S$ restricted to $[b,y^-]$. A change confined to $(y^-,\infty)$ leaves $y^-$ fixed while weakly raising $G_S$ elsewhere, so the greatest fixed point $y^+$ weakly rises. A change raising $H_S$ on $[b,y^-]$, or a larger $b$, raises $G_S$ on the iteration's range and weakly raises $y^-$.
\end{proof}

This is the standard threshold-cascade geometry \citep{granovetterThresholdModelsCollective1978}. The value of failure privacy is not total latent support but the mass beyond the exposure barrier that safe public expansion cannot reach. Part (iii) gives the comparative static: support above $y^-$ is invisible to decentralized expression, so a movement can have broad private backing and a small cascade when support is concentrated at requirements the early mass cannot bridge. The contract's contribution grows as support concentrates there. In the union application, these are the most-exposed workers, reachable only by the tunnel. Theorem~\ref{thm:selection} shows that the decentralized game selects $y^-$ rather than merely permitting a stop there. With ambient trust, agents may rely on promised follow-through and the public path may move beyond $y^-$. The model does not characterize the resulting endpoint.

\paragraph{Maximum protection shortfall.} Write
\[
\varsigma \;=\; \sup_{y\in[y^-,\,y^+]}\bigl(y-G_S(y)\bigr)^+,
\]
the largest amount by which protected mass falls short of public mass between $y^-$ and $y^+$. A movement that crosses by incremental public exposure must reach an intermediate roster at which at least $\varsigma$ units of public mass are borne by participants whom that roster does not protect. Reaching $y^+$ from below makes public mass pass through every intermediate level; where the shortfall peaks, at most $G_S(y)$ of that mass is protected. At least $\varsigma$ is therefore exposed along the path, which regret-free safety forbids and which explains why safe incremental expression halts at $\Cs$. Failure-private disclosure reaches $y^+$ with no such exposure. The shortfall is positive exactly when $G_S$ dips below the diagonal somewhere in $(y^-,y^+)$. A synchronized reveal avoids this incremental-path lower bound, but $\varsigma$ alone gives no upper bound on unsafe exposure in a particular realization: that depends on which agents complete. Proposition~\ref{prop:pact} instead bounds the probability of an unsafe realization from the completion law.

Real coalitions are atomic (each agent of positive, non-negligible size), and there the cascade and the destination are governed by different thresholds. With positive masses $a_i$, an agent can safely go public at existing public mass $y$ iff $y+a_i\ge\rho_i$, that is iff $y$ exceeds her \emph{activation threshold} $\check\rho_i:=\rho_i-a_i$; the cascade is therefore governed by the activation curve $K_S(y)=m\{i:\check\rho_i\le y\}$, while the tunnel destination $\Cp$ is still governed by final requirements $H_S(y)=m\{i:\rho_i\le y\}$. The two coincide in the nonatomic limit $a_i\to0$. The distinction has bite: a high-mass supporter can bootstrap the cascade despite a high requirement, because her own mass helps clear it.

As an illustration, take seed $b=1$ and consenters $\{x,y,w_1,w_2\}$ with $a_x=a_y=1$ and $a_{w_1}=a_{w_2}=1.5$ (so $m(S)=5$), requirements $\rho_x=2$, $\rho_y=3$, $\rho_{w_1}=\rho_{w_2}=6$; activation and requirement order coincide here ($\check\rho_x=1<\check\rho_y=2<\check\rho_w=4.5$). The cascade adds $x$ (public mass $b+a_x=2\ge\rho_x$), then $y$ (public mass $3\ge\rho_y$), then stalls: adding a $w$ would give public mass $4.5<6$. So $\Cs=\{x,y\}$, at public mass $y^-=3$. But $\Cp=S$, at public mass $y^+=b+m(S)=6\ge\rho_w$: the pair $(w_1,w_2)$ is safe only jointly, which unverified simultaneity cannot deliver and the tunnel can. The contribution is $m(\Cp)-m(\Cs)=5-2=3=y^+-y^-$.

\subsection{Information}\label{sec:design}

Audience beliefs $\mu$ enter through the protection families $\Pfam_i(\mu)$ and hence through $\Gamma_\mu$, $\Cs(\mu)$, and $\Cp(\mu)$. Information changes these protection families; conditional disclosure changes which fixed point can be reached at a fixed $\mu$.

\begin{remark}[Information and the path constraint]\label{cor:info}
At fixed $\mu$, a belief-only intervention that releases no named coalition leaves the safe-coalition fixed points unchanged: a public-only regret-free process remains bounded by $\Cs(\mu)$, while the social assurance contract implements $\Cp(\mu)$. The observation is immediate from the fixed-belief theorems and is recorded for the design discussion below.
\end{remark}

Corollary~\ref{cor:belief_only} distinguishes two cases. If an attainable belief makes a lone agent safe, information can start the public path. If no attainable belief does so, the same corollary shows that co-release remains necessary. Remark~\ref{cor:info} holds audience beliefs fixed when comparing the paths. The paper does not solve the joint design of information and the release path, nor does it claim that conditional disclosure generally dominates information design.

\subsection{Exogenous Conditioning Statistics: a Boundary Case}\label{sec:bbf}

\begin{remark}[The exogenous-statistic limit]\label{rem:bbf}
Threshold majority voting with disclosure conditions release on a statistic rather than on a protecting roster \citep{braghieriThresholdDisclosureCollective2026}. The realized vote share in that model is endogenous to participation and voting, so the proposition below does not formally nest it. The proposition instead isolates a stricter boundary: when the conditioning statistic is primitive and independent of who acts, the holding stage can coordinate release but cannot enlarge reach. Co-exposure-dependent safety restores roster composition, seed dependence, and a possible difference in feasible reach between cascade and tunnel.
\end{remark}

The following result is a boundary marker on this paper's primitives. It characterizes what disappears when safety is independent of the coalition and should not be read as a reduced form of an endogenous voting equilibrium.

\begin{proposition}[The exogenous-statistic limit]\label{prop:bbf}
Suppose each protection family conditions only on an exogenous statistic: there is a random variable $\sigma$, realized independently of the mechanism and of who is named, and thresholds $\sigma^\ast_i$ with $\Pfam_i=\{C\ni i:\sigma\ge\sigma^\ast_i\}$. Then for every consent set and seed: (i) $\Gamma(C)=C^\ast(\sigma):=\{i\in S:\sigma\ge\sigma^\ast_i\}$ for every $C$, the operator has the unique fixed point $C^\ast(\sigma)$, and $\Cs(S)=\Cp(S)=C^\ast(\sigma)$; (ii) outcomes are seed- and history-independent, pinned by $\sigma$ alone; (iii) failure privacy adds no reachability---a disclosure mechanism can at most coordinate arrival at $C^\ast(\sigma)$. Conversely, $\Cs\subsetneq\Cp$ requires protection to depend on co-exposure.
\end{proposition}

\begin{proof}
(i) For $C\ni i$, membership $C\in\Pfam_i$ holds iff $\sigma\ge\sigma^\ast_i$, independently of $C$'s composition; hence $\Gamma(C)=C^\ast(\sigma)$ for every $C$, the unique fixed point is $C^\ast(\sigma)$, and least and greatest coincide. Each $i\in C^\ast(\sigma)$ is safe alone, so $T(\varnothing)=C^\ast(\sigma)$: the cascade arrives in one round. (ii)--(iii) follow. For the converse, $\Cs\subsetneq\Cp$ requires some $i$ with $\Cp\in\Pfam_i$ and $\Cs\cup\{i\}\notin\Pfam_i$, impossible under composition-free membership.
\end{proof}

The comparison with \citet{braghieriThresholdDisclosureCollective2026} is therefore institutional rather than a nesting claim. Both papers study threshold-contingent disclosure. Their vote share is chosen in equilibrium; this proposition takes $\sigma$ as exogenous. Establishing a formal mapping would require carrying those endogenous voting choices into the coalition operator. The result here proves only that a fully exogenous, composition-free statistic cannot create a difference between the safe public path and the safe destination.

\section{Additional Applications and Scope}\label{sec:additional_apps}

\paragraph{Union organizing.} The retaliating audience is the employer; the protective audience is the labor board; the verifier is a confidentiality-bound certifier. The model isolates the \emph{exposure window} during which support is visible and retaliable. Open organizing is a cascade. Authorization cards signed privately and held until certification are a tunnel, often releasing a count to the board rather than a roster to the employer. This supplies protection through certified mass without guaranteeing anonymity; in a small unit the count can still reveal who signed (Proposition~\ref{prop:count}). The comparison between elections and card-based recognition is therefore a comparison between exposure windows, not simply between voting rules. Employer opposition is common in supervised campaigns \citep{bronfenbrennerNoHoldsBarred2009,mcnicholasUnlawfulUSEmployers2019}, while estimates of illegal organizer discharge remain contested \citep{schmittDroppingAxIllegal2009,lalondeHardTimesUnions1991,sherkTruthImproperFirings2007}. Neutrality and card-check agreements reduce management campaigning \citep{eatonUnionOrganizingNeutrality2001}. The application is imperfect because certification can complete an institutional outcome with a count, whereas strikes and walkouts require continued action after identities are known.

\paragraph{Dissent under repression.} The retaliating audience is the authority and the holding stage may be a diaspora administrator, a privately circulated declaration, or an encrypted escrow. Open dissent is the cascade of \citet{kuranPrivateTruthsPublic1997}; the institutional margin here is completed authorization, not merely information that others agree. The application requires two scope conditions. First, larger coalitions must be no less resilient, as in Section~\ref{sec:target}'s fight-or-fold benchmark. Second, signing must itself be appreciably safer than public expression. Under pervasive surveillance, the high-requirement agents the tunnel exists to reach may also have the highest signing exposure, shrinking the completed-authorization set $V$ and its ceiling $\Cp(V)$ toward or below $\Cs$. Belief-based turnout effects can also be strategic substitutes \citep{cantoniProtestsStrategicGames2019}; those effects operate through beliefs about participation, not through protection supplied by co-exposure.

\paragraph{Dual use: collusion.} A private holding stage can assemble harmful as well as beneficial coalitions. Firms contemplating a cartel may be unwilling to reveal intent before enough partners are committed. In that domain a large difference in feasible reach between cascade and tunnel is a social cost, and policy should attack the holding stage through subpoena, mandated disclosure, leniency, or infiltration. The mapping is not literal: cartel value comes from secrecy from regulators rather than public expression to a retaliating audience. Appendix~\ref{sec:value} gives a conditional welfare accounting.

\section{The Value of Reach: A Welfare Decomposition}\label{sec:value}

Feasible reach depends on entry, valid inputs, and a credible administrator. Greater reach need not improve welfare; its effect depends on which participants the mechanism enables to act. Failure privacy is dual-use: the same escrow that protects whistleblowers can protect price-fixers. Write the benchmark welfare measure as
\[
\Omega(C)=P(C)+X(C),
\]
where $P(C)=\sum_{i\in C}u_i(C)$ is participant surplus. It need not increase under arbitrary inclusion: a newly added member could contribute a negative payoff. It does increase along inclusions of self-protecting coalitions when each $u_i$ is nondecreasing in the coalition, because old members weakly gain and each new member has nonnegative payoff. Thus $P(\Cp)\ge P(\Cs)$. This payoff monotonicity is stronger than Assumption~\ref{ass:M}; upward closure of the protection family does not supply it. The term $X(C)$ is the externality of the released coalition on outsiders. The object of interest is
\[
\Delta\Omega=\Omega(\Cp)-\Omega(\Cs)=\underbrace{\Delta P}_{\ge0}+\underbrace{X(\Cp)-X(\Cs)}_{\text{ambiguous}} .
\]
The sign is deliberately unresolved. In an accountability application, truthful disclosures may create a positive externality; authentication and matching do not establish truth, so false or strategic reports can instead create harm. In a collusive application, added reach can impose losses on consumers or other outsiders. Nor does the difference between cascade and tunnel determine the sign: the externality depends on which people the tunnel reaches, not only on how many.

The displayed measure gives participant surplus unit weight and omits seed payoffs, signing and solicitation costs, delay, administration, and security costs. These omitted terms have no determinate net effect without a model of timing and payoffs. Giving participant surplus a domain-specific welfare weight $\eta\in[0,1]$ yields
\[
\Delta\Omega_\eta=\eta\,\Delta P+X(\Cp)-X(\Cs).
\]
This matters in extractive domains: cartel profit may be a transfer rather than value created, so a consumer-welfare calculation may put little or no weight on it. A large difference in reach is therefore not itself a welfare metric. The geometry determines feasible reach; an application must supply the externalities and omitted costs needed to value that reach.

\subsection{Scope of the Monotone Benchmark}\label{sec:scope}

The preceding results have a defined domain. The body's lattice needs monotone protection. Material-retaliation settings satisfy it only when additional public co-participants do not make incumbents less safe; material harm alone is not enough. The rest of this section treats environments in which monotone protection fails outright.

\paragraph{The nonmonotone frontier.} Two cases violate monotone protection. First, social-image models make exposure costs depend on audience beliefs and perceived norms \citep{benabouIncentivesProsocialBehavior2006,bursztynMisperceivedSocialNorms2020}. A co-signer whom the audience views negatively may then raise other members' exposure costs. Second, a member's record or vulnerability may lower the coalition's resilience $q(C)$ (Section~\ref{sec:target}), making the coalition easier to defeat. In either case, self-protecting coalitions need not be closed under union, and there may be no largest self-protecting roster. Accessibility then replaces the lattice.

Let $C_0$ be the irreversible seed and let $\Sigma\subseteq\{C:C_0\subseteq C\subseteq C_0\cup S\}$ be an arbitrary family of admissible public sets, with $C_0\in\Sigma$. Every nonseed member of an admissible set is protected there; the committed seed remains exempt, as in Section~\ref{sec:model}. A public step adds one agent and must leave the resulting set in $\Sigma$. The \emph{accessible kernel} $\mathcal K(C_0)$ is the set of coalitions that can be reached from $C_0$ through such safe one-agent steps.

Under monotone protection, Lemma~\ref{lem:reduction} makes safety after each individual completion enough to ensure safety under every realization. That equivalence fails here, so the next assumption strengthens Assumption~\ref{ass:U} for unverified public batches. It is an additional premise, not a consequence of nonmonotonicity.

\begin{assumption}[Batch admissibility]\label{ass:batch}
For an unverified public transition that attempts a set $E$, the admissible realization set contains, for every subset $E'\subseteq E$ and every ordering of $E'$, the realization in which exactly the members of $E'$ complete, one at a time, in that order. A device act releasing previously completed, held authorizations is instead governed by Assumption~\ref{ass:atomic}.
\end{assumption}

Treat $\Sigma$ as known. To implement a proposed coalition $C$, the administrator or protocol must know $\Sigma$, the seed $C_0$, and $C$. The proposition neither elicits protection sets nor chooses among incomparable admissible coalitions. Outside the monotone domain, there may be no greatest destination to select.

\begin{proposition}[Accessibility necessity]\label{thm:accessibility}
Maintain the consent-respecting act space and causal timing preceding Lemma~\ref{lem:dichotomy}, mechanisms as in Definition~\ref{def:mechanism}, and Assumptions~\ref{ass:atomic} and~\ref{ass:batch}. For any admissible family $\Sigma$ with irreversible seed $C_0$ as above: (i) a coalition is the outcome of some regret-free public-only process from $C_0$ if and only if it lies in the accessible kernel $\mathcal K(C_0)$; (ii) every $C\in\Sigma\setminus\mathcal K(C_0)$ requires a private conditional-release stage to implement, and holding authorizations from $C\setminus C_0$ before releasing those names in one atomic device act implements it. Failure privacy is therefore necessary and sufficient for exactly the admissible coalitions outside the kernel. When $\Sigma$ is generated by monotone protection (Assumption~\ref{ass:M}), $\max\mathcal K(C_0)=C_0\cup\Cs$ and $\max\Sigma=C_0\cup\Cp$, recovering Theorem~\ref{thm:necessity} with the seed made explicit.
\end{proposition}

\begin{proof}
(i) A regret-free public-only process exposes names irreversibly, and its transitions condition only on completed exposures. Fix any transition that newly attempts a set $E$ of agents. Because no held authorization gates a public-only transition, it is an unverified public batch governed by Assumption~\ref{ass:batch}. Regret-freeness must hold along every admissible realization, so each prefix of each completion order, added to the current public set, lies in $\Sigma$. Expanding each realized batch transition into one such safe order and concatenating across transitions yields a unit-increment chain from $C_0$ to the outcome. Hence the outcome lies in $\mathcal K(C_0)$. Conversely, a chain witnessing $C\in\mathcal K(C_0)$ realizes $C$ by singleton attempts, and every prefix remains in $\Sigma$, so the process is regret-free. (ii) If $C\in\Sigma\setminus\mathcal K(C_0)$, no unit-increment safe public chain reaches $C$. By (i), a transition leaving the kernel cannot consist only of unverified public attempts. In the maintained consent-respecting act space, any multi-name event that eliminates the partial-completion realizations must be one device act resting on completed, still-unattributed authorizations: Lemma~\ref{lem:holding}. Thus any regret-free implementation of $C$ contains a private conditional-release stage. Conversely, collect completed authorizations from every member of $C\setminus C_0$ while keeping them unattributed and release those names through one device act. Its failure leaves $C_0$ public and its completion makes $C$ public; both lie in $\Sigma$, and Assumption~\ref{ass:atomic} rules out a partial roster. This implements $C$. Under Assumption~\ref{ass:M}, restoring the suppressed seed identifies the maximal accessible and admissible public sets as $C_0\cup\Cs$ and $C_0\cup\Cp$.
\end{proof}

\begin{proposition}[Intractability of the optimal coalition]\label{thm:nphard}
An instance consists of a finite set $S$, a Boolean circuit $Q_I$ with $|S|$ input bits such that $C\in\Sigma_I$ iff $Q_I(\mathbf 1_C)=1$, nonnegative integer weights $x_i$, and a target $k$, with all integers binary encoded. Deciding whether some $C\in\Sigma_I$ has $\sum_{i\in C}x_i\ge k$ (in particular, whether some $C\in\Sigma_I$ has $|C|\ge k$) is NP-complete, and computing a maximum-weight admissible coalition is NP-hard.
\end{proposition}

The circuit is a compact membership representation; an explicit enumeration of the family, which can be exponential in $|S|$, is never formed. Both the circuit and the objective weights are supplied to the planner. The result does not provide a way to learn either input from prospective members.

\begin{proof}
A coalition's incidence vector is a polynomial certificate: circuit evaluation verifies $C\in\Sigma_I$, and binary addition verifies the weight bound, so the problem is in NP. Hardness is the standard reduction from \textsc{Independent Set}. Given $G=(V,E)$, set $S=V$, use unit weights, and construct
\[
Q_G(z)=\bigwedge_{\{u,v\}\in E}(\neg z_u\lor\neg z_v).
\]
The circuit has size $O(|V|+|E|)$ and accepts exactly the independent sets of $G$---equivalently, the protection construction $\Pfam_i=\{C\ni i:\text{no neighbor of }i\text{ lies in }C\}$. Thus an accepted coalition of weight at least $k$ exists iff $G$ has an independent set of size at least $k$. The weighted optimization statement embeds \textsc{Maximum-Weight Independent Set}.
\end{proof}

\begin{proposition}[A tractable size-and-average-type subclass]\label{prop:scalar_image}
Suppose agent $i$ is safe in $C$ iff $|C|\ge n_i$ and the average type $\bar\tau(C)=\frac{1}{|C|}\sum_{j\in C}\tau_j\ge s$ for a common requirement $s$ and individual size requirements $n_i$. Then a maximum-cardinality self-protecting coalition is computable in $O(n^2)$ time. If, in addition, social weight is nondecreasing in type---the \emph{aligned} case---the maximum-weight self-protecting coalition is computable in the same way. Without alignment, with rational $s,\tau_i$ and integer social weights and target $W$ encoded in binary, deciding whether some self-protecting coalition of a fixed size has weight at least $W$ is an exact-cardinality knapsack and is weakly NP-hard; no polynomial bound is claimed. Restricting the nonmonotonicity to coalition size and average type thus restores, in the aligned case, the tractability lost in Proposition~\ref{thm:nphard}.
\end{proposition}

\begin{proof}
A coalition of size $m$ is self-protecting iff all its members satisfy $n_i\le m$---so they are drawn from $A_m=\{i:n_i\le m\}$ with $|A_m|\ge m$---and $\bar\tau\ge s$. Among size-$m$ subsets of $A_m$, average type is maximized by the $m$ highest-type members; if even that subset has $\bar\tau<s$, no size-$m$ self-protecting coalition exists, and otherwise it is a self-protecting coalition of size $m$. Sorting types once costs $O(n\log n)$; for each $m$, one pass over the sorted list collects the $m$ highest-type members of $A_m$ and their running sum, an $O(n)$ scan per size and $O(n^2)$ in total, and the scan over $m=1,\dots,n$ returns the largest feasible $m$. When social weight is monotone in type, the same $m$ highest-type members also maximize total weight among size-$m$ subsets of $A_m$ while being the easiest to satisfy the average constraint, so the identical scan returns the maximum-weight coalition. For the unaligned boundary, reduce exact-cardinality knapsack with costs $c_i$, values $x_i$, budget $B$, and target cardinality $m$: set every $n_i=1$, choose $L\ge\max_i c_i$, put $\tau_i=L-c_i$ and $s=L-B/m$, and use $x_i$ as social weight. Then a size-$m$ coalition clears $\bar\tau\ge s$ iff its total cost is at most $B$, and its weight is the knapsack value. The binary-encoded problem is therefore weakly NP-hard (and pseudo-polynomial by the usual dynamic program), so the stated polynomial bound is claimed only for the aligned case.
\end{proof}

Outside the monotone domain, implementation is governed by accessibility rather than a lattice, and the planner's problem is generally intractable. The reduction is standard; the result marks the boundary of the tractable benchmark. Tractability returns in the size-and-average-type subclass of Proposition~\ref{prop:scalar_image} only for maximum cardinality or for supplied objective weights aligned with type. These results still do not select a unique admissible coalition. Choosing among incomparable coalitions requires the planner's objective and knowledge of the protection constraints.

\ifSubfilesClassLoaded{%
  \bibliographystyle{aea}
  \bibliography{safe_coalitions}
}{ }

\end{document}
